# Supplementary material for: Unlocking Scientific Concepts: How Effective Are LLM-Generated Analogies for Student Understanding and Classroom Practice?
Source: arXiv:2502.16895 source file (2025-02-24)
Supplement: Supplementary file 1 [file 090appendix.tex]

\newpage
\section*{Appendix}
\subsection{Details about Analogy Generation from LLMs}
\input{table/full_prompt}
\subsubsection{Plain Analogy Generation}
To align with the educational process for students, we requested the most advanced LLM, \ie, GPT-4o~\cite{openai_gpt-4_2023}, to generate free-form analogies for each scientific concept. We adhered to the prompt settings described in \cite{bhavya-etal-2022-analogy} for the generation process. 
Specifically, to facilitate more effective analogy generation by GPT-4o, we incorporated principles from analogy cognition theory~\cite{hesse1959defining,gentner1983structure,gentner2017analogy} into the instruction prompt. Additionally, we provided GPT-4o with textbook content relevant to the scientific concepts to tailor the analogies to students' learning progress.
We did not include examples in the instruction prompt because there is no high-quality analogy dataset in the educational domain from which students can learn. 
Examples could induce bias in GPT-4o~\cite{pmlr-v139-zhao21c}, thereby degrading the generalization of analogy generation.

\subsubsection{Error Annotation for Generated Analogy}
Based on the prompt in step 2, we set the temperature to 0.7 for GPT-4o and generated three analogies for each concept. Then, three authors served as annotators to evaluate the quality of the generated analogies by annotating the errors. Initially, the annotators followed two common categories of error classification typically used in LLM outputs~\cite{jang-etal-2022-becel,gekhman-etal-2023-trueteacher,chuang2024dola}: 1) Factual Accuracy: the appropriateness of the analogies for the given concept; 2) Consistency: the coherence of objects within the analogies. 
The three annotators independently applied this classification to their annotations. After annotating 10 analogies, a discussion about error codes and annotations was conducted. Following three discussions, the annotators categorized the error codes into five types: the first three are factual errors, while the last two are inconsistency errors.
\begin{itemize}
    \item \textbf{Concept Paradox}: The analogy inaccurately represents the scientific concept, conflicting with established physical phenomena and commonsense knowledge.
    \item \textbf{Analogy Object Paradox}: The objects within the analogy do not align with physical laws or commonsense knowledge.
    \item \textbf{Inappropriate Analogy}: The analogy fails to accurately mirror the concept, leading to misconceptions.
    \item \textbf{Object Confusion}: The same analogy objects are assigned different roles or functions across various contexts.
    \item \textbf{Logical Contradiction}: The syntax within a sentence or paragraph contradicts itself.
\end{itemize}

After repeated discussions, the inter-rater reliability among annotators reached Fleiss' Kappa of 0.83 for Analogy Object Paradox, 0.94 for Object Confusion, and 1 for the remaining error codes.
As shown in the first row of Table.~\ref{tab:error_rates}.
Despite the powerful capabilities of GPT-4o, it fails to generate appropriate and satisfactory analogies for scientific concepts with our initial principles. 
Specifically, concerning the factual aspect, GPT-4o attempts to produce analogies that adhere to physical logic. 
However, the objects within these analogies often contradict physical laws or commonsense knowledge, resulting in errors related to the analogy objects.

Moreover, in the generated analogies, the same objects are inconsistently assigned different roles or functions in various contexts, indicating that GPT-4o suffers from object confusion.
For example, when generating analogies for the photoelectric effect, GPT-4o uses a trampoline. 
In this analogy, the trampoline represents the metal surface, and children represent electrons. 
The model initially makes an analogy between the force with which a worker presses the trampoline and the frequency of light, \eg, \textit{``First, if someone presses down on a diving board with a very small force (low-frequency light), the diving board will not have enough elasticity to bounce you back up.''}
However, in later descriptions, this force is equated to light intensity, \eg, \textit{``The greater the force applied (the higher the intensity of light), the more people will be bounced off the diving board in a given period.''}.

\subsubsection{Analogy Generation with Revised Prompt and Second Round of Error Annotation}
In Step 3, we discovered that GPT-4o cannot generate appropriate analogies directly, as it produces several errors. 
Therefore, we refined the prompt by incorporating new principles to guide GPT-4o in avoiding these errors, enhancing the quality of the generated analogies. 
Table~\ref{tab:instruction_prompt_full} (II) details the revised prompt template.
The three annotators applied the error codes used in Step 3 to the analogies generated in this round.
After two rounds of discussions, the inter-rater reliability among annotators reached Fleiss' Kappa of 0.84 for Analogy Object Paradox, 0.94 for Inappropriate Analogy, 0.92 for Object Confusion, and 1 for the remaining error codes.
Based on Table~\ref{tab:error_rates}, we can find that the revised prompt enhances the coherence of objects within analogies, thereby minimizing confusion and logical contradictions during generation. 
However, to accurately identify analogous relationships, the model may force objects to conform to patterns that contradict physical laws or common sense, thereby intensifying the analogy object paradox.

\subsubsection{Automatic Analogy Selection from LLMs}

From step 4, it is evident that the model is still prone to errors despite providing clear and instructive guidelines. 
Previous research in the AI community has demonstrated that models can select the optimal result from multiple outputs through a process known as self-correction~\cite{pan2023automatically,yuan-etal-2023-distilling,liu2024large}. 
Therefore, we allowed GPT-4o to choose the best result according to the guidelines from three analogies generated for each concept. 
The chosen prompts are displayed in Table~\ref{tab:instruction_prompt_full} (III). 
Results in Table~\ref{tab:error_rates} show that enabling the model to self-correct enhances the accuracy of the analogies. 
However, the model struggles with issues such as object confusion. 
We hypothesize that this difficulty arises because the objects in the analogies are described in disparate text sections, requiring the model to use contextual cues for differentiation. 
This necessitates a robust capability for understanding long contexts~\cite{li2024can}. 

\subsection{Principle Generation in System Workflow}
In our practical system, we adopt GPT-4o to summarize new principles from comments on the three analogies and add them to the principles list (\textbf{G2}).
The prompt template is: 
\begin{tcolorbox}[title=The prompt template of principle generation, mybox]
Based on the analogy you generated, the teacher's suggestion is:
```
{teacher_suggestion}.
```
Now, you do not need to generate new analogies, but instead, you need to generate more new guidelines to enrich the original ones based on the teacher's suggestion.

Original guidelines:
- The similarity between the objects in the analogy and those in the scientific concept should be minimal.  
- The relationships in the analogy and the scientific concept should be highly similar. 
- The analogy should use objects that students are very familiar with from everyday experiences. 
- The analogy should accurately identify similar relationships with the scientific concept and avoid forcing non-existent similarities.  
- The objects in the analogy and the scientific concept should align with scientific laws and commonsense knowledge. 
- An object in the analogy cannot have different roles or functions in different contexts.  
- The logic within a sentence or paragraph should not be self-contradictory.  
{current_strategies}
{current_guidelines}

Remember:  
1. The new guidelines should be different from the original guidelines.  
2. The new guidelines should be generated based on the teacher's suggestion.  
The format is as follows:
```
New guidelines:
- xxx
- xxx
- xxx
....
```
New guidelines:
\end{tcolorbox}
